# Supplementary material for: Hidden Supersymmetry May Imply Duality Invariance
Source: arXiv:1303.5663 ancillary file (2013-03-22)
Supplement: Supplementary file 1 [file ancillaryNotes.pdf]

# Notes on Direct Verification of Duality

John Joseph M. Carrasco and Renata Kallosh

<sup>a</sup>Stanford Institute for Theoretical Physics and Department of Physics,  
Stanford University, Stanford, CA 94305, USA

## I. EXPLICIT FORM OF ACTION AND MANIFEST DUALITY SATISFACTION.

Through the first duality untested order ( $\mathcal{W}^{10}$ ) the BIK action [1] is

$$\mathcal{S}_{\text{BI}} = \mathcal{S}_{\text{free}} + \mathcal{S}_{\text{int},10} \quad (1.1)$$

where the interaction term is given (up to total derivatives):

$$\begin{aligned} \mathcal{S}_{\text{int},10} = \int d^{12}\mathcal{Z} & \left\{ \frac{1}{8} \mathcal{W}^2 \bar{\mathcal{W}}^2 \lambda + \lambda^2 \left( \frac{1}{72} \mathcal{W}^3 \square [\bar{\mathcal{W}}^3] + \frac{1}{16} \mathcal{W}^2 \bar{\mathcal{W}}^2 \mathcal{D}^4 [\mathcal{W}^2] + \frac{1}{16} \mathcal{W}^2 \bar{\mathcal{W}}^2 \bar{\mathcal{D}}^4 [\bar{\mathcal{W}}^2] \right) \right. \\ & + \lambda^3 \left( \frac{\mathcal{W}^4 \square [\square [\bar{\mathcal{W}}^4]]}{1152} + \frac{1}{48} \mathcal{W}^3 \square [\bar{\mathcal{W}}^3 \mathcal{D}^4 [\mathcal{W}^2]] + \frac{1}{48} \bar{\mathcal{W}}^3 \square [\mathcal{W}^3 \bar{\mathcal{D}}^4 [\bar{\mathcal{W}}^2]] + \frac{1}{32} \mathcal{W}^2 \bar{\mathcal{W}}^2 \mathcal{D}^4 [\mathcal{W}^2]^2 \right. \\ & \quad \left. + \frac{3}{32} \mathcal{W}^2 \bar{\mathcal{W}}^2 \mathcal{D}^4 [\mathcal{W}^2] \bar{\mathcal{D}}^4 [\bar{\mathcal{W}}^2] + \frac{1}{32} \mathcal{W}^2 \bar{\mathcal{W}}^2 \bar{\mathcal{D}}^4 [\bar{\mathcal{W}}^2]^2 \right) \\ & + \lambda^4 \left( -\frac{\mathcal{W}^5 \square [\square [\square [\bar{\mathcal{W}}^5]]]}{28800} + \frac{1}{576} \bar{\mathcal{W}}^4 \square [\square [\mathcal{W}^4 \bar{\mathcal{D}}^4 [\bar{\mathcal{W}}^2]]] + \frac{1}{576} \square [\mathcal{W}^4] \square [\bar{\mathcal{W}}^4 \mathcal{D}^4 [\mathcal{W}^2]] + \frac{1}{48} \mathcal{W}^3 \square [\bar{\mathcal{W}}^3 \mathcal{D}^4 [\mathcal{W}^2]^2] \right. \\ & + \frac{1}{48} \bar{\mathcal{W}}^3 \square [\mathcal{W}^3 \bar{\mathcal{D}}^4 [\bar{\mathcal{W}}^2]^2] + \frac{1}{36} \bar{\mathcal{W}}^3 \square [\mathcal{W}^3 \bar{\mathcal{D}}^4 [\bar{\mathcal{W}}^2]] \mathcal{D}^4 [\mathcal{W}^2] + \frac{1}{64} \mathcal{W}^2 \bar{\mathcal{W}}^2 \mathcal{D}^4 [\mathcal{W}^2]^3 + \frac{1}{576} \bar{\mathcal{W}}^4 \square [\mathcal{W}^3] \mathcal{D}^4 [\square [\mathcal{W}^3]] \\ & + \frac{1}{16} \mathcal{W}^2 \bar{\mathcal{W}}^2 \mathcal{D}^4 [\mathcal{W}^2]^2 \bar{\mathcal{D}}^4 [\bar{\mathcal{W}}^2] + \frac{1}{32} \mathcal{W}^2 \bar{\mathcal{W}}^2 \mathcal{D}^4 [\mathcal{W}^2 \bar{\mathcal{D}}^4 [\bar{\mathcal{W}}^2]] \bar{\mathcal{D}}^4 [\bar{\mathcal{W}}^2] + \frac{1}{16} \mathcal{W}^2 \bar{\mathcal{W}}^2 \mathcal{D}^4 [\mathcal{W}^2] \bar{\mathcal{D}}^4 [\bar{\mathcal{W}}^2]^2 \\ & \quad \left. + \frac{1}{64} \mathcal{W}^2 \bar{\mathcal{W}}^2 \bar{\mathcal{D}}^4 [\bar{\mathcal{W}}^2]^3 + \frac{1}{576} \mathcal{W}^4 \square [\bar{\mathcal{W}}^3] \bar{\mathcal{D}}^4 [\square [\bar{\mathcal{W}}^3]] + \frac{1}{32} \mathcal{W}^2 \bar{\mathcal{W}}^2 \mathcal{D}^4 [\mathcal{W}^2] \bar{\mathcal{D}}^4 [\bar{\mathcal{W}}^2 \mathcal{D}^4 [\mathcal{W}^2]] \right) \Big\} \quad (1.2) \end{aligned}$$

One can directly verify the duality-covariance of the action through  $\mathcal{W}^{10}$  by checking the self-duality constraint:

$$\int d^8 \mathcal{Z} (\mathcal{W}^2 + \mathcal{M}^2) - \int d^8 \bar{\mathcal{Z}} (\bar{\mathcal{W}}^2 + \bar{\mathcal{M}}^2) = 0, \quad (1.3)$$

using  $i\mathcal{M} \equiv 4 \frac{d}{d\mathcal{W}} \mathcal{S}[\mathcal{W}, \bar{\mathcal{W}}]$ . One simply brings the difference between the two integrands from  $\int d^8 \mathcal{Z}$  and  $\int d^8 \bar{\mathcal{Z}}$  respectively under the same  $\int d^{12} \mathcal{Z}$  integral by using  $\int d^8 \mathcal{Z} \bar{\mathcal{D}}^4 (X) - \int d^8 \bar{\mathcal{Z}} \mathcal{D}^4 (Y) = \int d^{12} \mathcal{Z} (X - Y)$ . One can group the resulting integrand  $(X - Y)$  by powers of  $\lambda$ ,  $\square$ ,  $\bar{\mathcal{D}}^4$ , and  $\mathcal{D}^4$ . From the manifestly supersymmetric BIK action we have sufficient data to analyze that  $(X - Y)$  vanishes through order  $\lambda^4$  – any higher power of  $\lambda$  would require specifying  $\lambda^{n \geq 5}$  terms in the action. Here we sketch all such groupings relevant to  $\mathcal{S}_{\text{int},10}$ . Specially:

$$0 = \frac{1}{3} I_2 + \frac{1}{36} I_{3a} + \frac{1}{2} I_{3b} + 2I_{3c} + \frac{1}{720} I_{4a} + \frac{1}{12} I_{4b} + \frac{1}{12} I_{4c} + \frac{1}{6} I_{4d} + \frac{1}{6} I_{4e} + \frac{1}{18} I_{4f} + \frac{1}{18} I_{4g} + \frac{1}{18} I_{4h} + \frac{1}{2} I_{4i} + \frac{1}{2} I_{4j} \quad (1.4)$$

For duality to be satisfied, each such group could be expected to vanish independently (under boundary conditions of the integration), and it is straightforward, if perhaps somewhat tedious, to verify that it in fact does. Here we show, e.g., one of the terms that had to vanish.

$$\begin{aligned} I_{4i} = \lambda^4 \int d^{12} \mathcal{Z} & \left( +7 \mathcal{W}^2 \bar{\mathcal{W}}^2 \mathcal{D}^4 [\mathcal{W}^2]^2 \bar{\mathcal{D}}^4 [\bar{\mathcal{W}}^2] - 4 \mathcal{W}^2 \bar{\mathcal{W}}^2 \mathcal{D}^4 [\mathcal{W}^2] \mathcal{D}^4 [\mathcal{W}^2 \bar{\mathcal{D}}^4 [\bar{\mathcal{W}}^2]] \right. \\ & \left. + 3 \mathcal{W}^2 \bar{\mathcal{W}}^2 \mathcal{D}^4 [\mathcal{W}^2 \bar{\mathcal{D}}^4 [\bar{\mathcal{W}}^2 \mathcal{D}^4 [\mathcal{W}^2]]] - 3 \mathcal{W}^2 \bar{\mathcal{W}}^2 \mathcal{D}^4 [\mathcal{W}^2] \bar{\mathcal{D}}^4 [\bar{\mathcal{W}}^2 \mathcal{D}^4 [\mathcal{W}^2]] - 3 \mathcal{W}^2 \bar{\mathcal{W}}^2 \bar{\mathcal{D}}^4 [\bar{\mathcal{W}}^2 \mathcal{D}^4 [\mathcal{W}^2]^2] \right) \quad (1.5) \end{aligned}$$

One can note that the types of cancellations involve rather trivial integration by parts identities. This is largely the case throughout. The rest of the expressions follow:

$$I_2 = \lambda^2 \int d^{12} \mathcal{Z} \left( \bar{\mathcal{W}}^3 \square [\mathcal{W}^3] - \mathcal{W}^3 \square [\bar{\mathcal{W}}^3] \right) \quad (1.6)$$

$$I_{3a} = \lambda^3 \int d^{12} \mathcal{Z} \left( \bar{\mathcal{W}}^4 \square [\square [\mathcal{W}^4]] - \mathcal{W}^4 \square [\square [\bar{\mathcal{W}}^4]] \right) \quad (1.7)$$

$$I_{3b} = \lambda^3 \int d^{12} \mathcal{Z} \left( -\mathcal{W}^3 \square [\bar{\mathcal{W}}^3 \mathcal{D}^4 [\mathcal{W}^2]] + \mathcal{W}^2 \bar{\mathcal{W}}^3 \mathcal{D}^4 [\square [\mathcal{W}^3]] \right) \quad (1.8)$$

$$I_{3c} = \lambda^3 \int d^{12} \mathcal{Z} \left( \mathcal{W}^2 \bar{\mathcal{W}}^2 \mathcal{D}^4 [\mathcal{W}^2 \bar{\mathcal{D}}^4 [\bar{\mathcal{W}}^2]] - \mathcal{W}^2 \bar{\mathcal{W}}^2 \bar{\mathcal{D}}^4 [\bar{\mathcal{W}}^2 \mathcal{D}^4 [\mathcal{W}^2]] \right) \quad (1.9)$$

$$I_{4a} = \lambda^4 \int d^{12} \mathcal{Z} \left( -\bar{\mathcal{W}}^5 \square [\square [\square [\mathcal{W}^5]]] + \mathcal{W}^5 \square [\square [\square [\bar{\mathcal{W}}^5]]] \right) \quad (1.10)$$

$$I_{4b} = \lambda^4 \int d^{12} \mathcal{Z} \left( -\mathcal{W}^3 \square [\bar{\mathcal{W}}^4 \mathcal{D}^4 [\square [\mathcal{W}^3]]] + \bar{\mathcal{W}}^4 \square [\mathcal{W}^3] \mathcal{D}^4 [\square [\mathcal{W}^3]] \right) \quad (1.11)$$

$$I_{4c} = \lambda^4 \int d^{12} \mathcal{Z} \left( \bar{\mathcal{W}}^3 \square [\mathcal{W}^4 \bar{\mathcal{D}}^4 [\square [\bar{\mathcal{W}}^3]]] - \mathcal{W}^4 \square [\bar{\mathcal{W}}^3] \bar{\mathcal{D}}^4 [\square [\bar{\mathcal{W}}^3]] \right) \quad (1.12)$$

$$I_{4d} = \lambda^4 \int d^{12} \mathcal{Z} \left( -3\mathcal{W}^3 \square [\bar{\mathcal{W}}^3 \mathcal{D}^4 [\mathcal{W}^2]^2] + 7\bar{\mathcal{W}}^3 \square [\mathcal{W}^3] \mathcal{D}^4 [\mathcal{W}^2]^2 - 4\mathcal{W}^2 \bar{\mathcal{W}}^3 \mathcal{D}^4 [\mathcal{W}^2] \mathcal{D}^4 [\square [\mathcal{W}^3]] \right) \quad (1.13)$$

$$I_{4e} = \lambda^4 \int d^{12} \mathcal{Z} \left( 3\bar{\mathcal{W}}^3 \square [\mathcal{W}^3 \bar{\mathcal{D}}^4 [\bar{\mathcal{W}}^2]^2] - 7\mathcal{W}^3 \square [\bar{\mathcal{W}}^3] \bar{\mathcal{D}}^4 [\bar{\mathcal{W}}^2]^2 + 4\mathcal{W}^3 \bar{\mathcal{W}}^2 \bar{\mathcal{D}}^4 [\bar{\mathcal{W}}^2] \bar{\mathcal{D}}^4 [\square [\bar{\mathcal{W}}^3]] \right) \quad (1.14)$$

$$I_{4f} = \lambda^4 \int d^{12} \mathcal{Z} \left( -\mathcal{W}^4 \square [\square [\bar{\mathcal{W}}^4 \mathcal{D}^4 [\mathcal{W}^2]]] + \mathcal{W}^2 \bar{\mathcal{W}}^4 \mathcal{D}^4 [\square [\square [\mathcal{W}^4]]] \right) \quad (1.15)$$

$$I_{4g} = \lambda^4 \int d^{12} \mathcal{Z} \left( \bar{\mathcal{W}}^4 \square [\square [\mathcal{W}^4 \bar{\mathcal{D}}^4 [\bar{\mathcal{W}}^2]]] - \mathcal{W}^4 \bar{\mathcal{W}}^2 \bar{\mathcal{D}}^4 [\square [\square [\bar{\mathcal{W}}^4]]] \right) \quad (1.16)$$

$$\begin{aligned} I_{4h} = \lambda^4 \int d^{12} \mathcal{Z} & \left( 13\mathcal{W}^2 \bar{\mathcal{W}}^3 \mathcal{D}^4 [\square [\mathcal{W}^3 \bar{\mathcal{D}}^4 [\bar{\mathcal{W}}^2]]] - 13\mathcal{W}^3 \bar{\mathcal{W}}^2 \bar{\mathcal{D}}^4 [\square [\bar{\mathcal{W}}^3 \mathcal{D}^4 [\mathcal{W}^2]]] \right. \\ & + 6\bar{\mathcal{W}}^3 \square [\mathcal{W}^3] \mathcal{D}^4 [\mathcal{W}^2 \bar{\mathcal{D}}^4 [\bar{\mathcal{W}}^2]] - 6\mathcal{W}^2 \bar{\mathcal{W}}^2 \bar{\mathcal{D}}^4 [\bar{\mathcal{W}}^3 \mathcal{D}^4 [\square [\mathcal{W}^3]]] \\ & \left. + 6\mathcal{W}^2 \bar{\mathcal{W}}^2 \mathcal{D}^4 [\mathcal{W}^3 \bar{\mathcal{D}}^4 [\square [\bar{\mathcal{W}}^3]]] - 6\mathcal{W}^3 \square [\bar{\mathcal{W}}^3] \bar{\mathcal{D}}^4 [\bar{\mathcal{W}}^2 \mathcal{D}^4 [\mathcal{W}^2]] \right) \quad (1.17) \end{aligned}$$

$$\begin{aligned} I_{4j} = \lambda^4 \int d^{12} \mathcal{Z} & \left( -7\mathcal{W}^2 \bar{\mathcal{W}}^2 \mathcal{D}^4 [\mathcal{W}^2] \bar{\mathcal{D}}^4 [\bar{\mathcal{W}}^2]^2 + 4\mathcal{W}^2 \bar{\mathcal{W}}^2 \bar{\mathcal{D}}^4 [\bar{\mathcal{W}}^2] \bar{\mathcal{D}}^4 [\bar{\mathcal{W}}^2 \mathcal{D}^4 [\mathcal{W}^2]] \right. \\ & \left. - 3\mathcal{W}^2 \bar{\mathcal{W}}^2 \bar{\mathcal{D}}^4 [\bar{\mathcal{W}}^2 \mathcal{D}^4 [\mathcal{W}^2 \bar{\mathcal{D}}^4 [\bar{\mathcal{W}}^2]]] + 3\mathcal{W}^2 \bar{\mathcal{W}}^2 \mathcal{D}^4 [\mathcal{W}^2 \bar{\mathcal{D}}^4 [\bar{\mathcal{W}}^2]] \bar{\mathcal{D}}^4 [\bar{\mathcal{W}}^2] + 3\mathcal{W}^2 \bar{\mathcal{W}}^2 \mathcal{D}^4 [\mathcal{W}^2 \bar{\mathcal{D}}^4 [\bar{\mathcal{W}}^2]^2] \right) \quad (1.18) \end{aligned}$$

It is straightforward to confirm that they are all total derivatives, for example by trivial operation of the identities described in Appendix C of [2].

## II. ACTION GENERATED BY SOURCES OF DEFORMATION

The generically self-dual interaction action generated by the sources of deformation given in the main text and the procedure of [2] (up to total derivatives) is as follows:

$$\begin{aligned}
S_{int,\lambda-\lambda^4} = \int d^{12}\mathcal{Z} \Bigg\{ & -2\lambda a_0 \mathcal{W}^2 \bar{\mathcal{W}}^2 + \lambda^2 \left( 16\mathcal{W}^2 \bar{\mathcal{W}}^2 \mathcal{D}^4 [\mathcal{W}^2] a_0^2 + 16\mathcal{W}^2 \bar{\mathcal{W}}^2 \bar{\mathcal{D}}^4 [\bar{\mathcal{W}}^2] a_0^2 - 8\mathcal{W}^3 \square [\bar{\mathcal{W}}^3] a_1 \right) \\
& + \lambda^3 \left( -128\mathcal{W}^2 \bar{\mathcal{W}}^2 \mathcal{D}^4 [\mathcal{W}^2]^2 a_0^3 - 128\mathcal{W}^2 \bar{\mathcal{W}}^2 \bar{\mathcal{D}}^4 [\bar{\mathcal{W}}^2]^2 a_0^3 + 192\mathcal{W}^3 \square [\bar{\mathcal{W}}^3 \mathcal{D}^4 [\mathcal{W}^2]] a_0 a_1 \right. \\
& + 192\bar{\mathcal{W}}^3 \square [\mathcal{W}^3 \bar{\mathcal{D}}^4 [\bar{\mathcal{W}}^2]] a_0 a_1 - 32\mathcal{W}^4 \square [\square [\bar{\mathcal{W}}^4]] a_2 - 32\mathcal{W}^2 \bar{\mathcal{W}}^2 \mathcal{D}^4 [\mathcal{W}^2] \bar{\mathcal{D}}^4 [\bar{\mathcal{W}}^2] (16a_0^3 + a_3) \Bigg) \\
& + \lambda^4 \left( 1024\mathcal{W}^2 \bar{\mathcal{W}}^2 \mathcal{D}^4 [\mathcal{W}^2]^3 a_0^4 + 1024\mathcal{W}^2 \bar{\mathcal{W}}^2 \bar{\mathcal{D}}^4 [\bar{\mathcal{W}}^2]^3 a_0^4 - 3072\mathcal{W}^3 \square [\bar{\mathcal{W}}^3 \mathcal{D}^4 [\mathcal{W}^2]^2] a_0^2 a_1 \right. \\
& - 3072\bar{\mathcal{W}}^3 \square [\mathcal{W}^3 \bar{\mathcal{D}}^4 [\bar{\mathcal{W}}^2]^2] a_0^2 a_1 + 576\bar{\mathcal{W}}^4 \square [\mathcal{W}^3] \mathcal{D}^4 [\square [\mathcal{W}^3]] a_1^2 + 576\mathcal{W}^4 \square [\bar{\mathcal{W}}^3] \bar{\mathcal{D}}^4 [\square [\bar{\mathcal{W}}^3]] a_1^2 \\
& + 1024\mathcal{W}^4 \square [\square [\bar{\mathcal{W}}^4 \mathcal{D}^4 [\mathcal{W}^2]]] a_0 a_2 + 1024\bar{\mathcal{W}}^4 \square [\square [\mathcal{W}^4 \bar{\mathcal{D}}^4 [\bar{\mathcal{W}}^2]]] a_0 a_2 \\
& + 512\mathcal{W}^2 \bar{\mathcal{W}}^2 \bar{\mathcal{D}}^4 [\bar{\mathcal{W}}^2] a_0 \left( \mathcal{D}^4 [\mathcal{W}^2 \bar{\mathcal{D}}^4 [\bar{\mathcal{W}}^2]] (8a_0^3 + a_3) + \mathcal{D}^4 [\mathcal{W}^2] \bar{\mathcal{D}}^4 [\bar{\mathcal{W}}^2] (12a_0^3 + a_3) \right) \\
& + 512\mathcal{W}^2 \bar{\mathcal{W}}^2 \mathcal{D}^4 [\mathcal{W}^2] a_0 \left( \bar{\mathcal{D}}^4 [\bar{\mathcal{W}}^2 \mathcal{D}^4 [\mathcal{W}^2]] (8a_0^3 + a_3) + \mathcal{D}^4 [\mathcal{W}^2] \bar{\mathcal{D}}^4 [\bar{\mathcal{W}}^2] (12a_0^3 + a_3) \right) \\
& \left. - \frac{1}{4}\mathcal{W}^5 \square [\square [\square [\bar{\mathcal{W}}^5]]] a_4 + \frac{1}{4}\bar{\mathcal{W}}^3 \square [\mathcal{W}^3 \bar{\mathcal{D}}^4 [\bar{\mathcal{W}}^2]] \mathcal{D}^4 [\mathcal{W}^2] (-18432a_0^2 a_1 - a_5) \right) \Bigg\} \quad (2.1)
\end{aligned}$$

Using  $\vec{a}_{0-5} = (-2^{-4}, -2^{-6} 3^{-2}, -2^{-12} 3^{-2}, 2^{10}, 2^{-5} 3^{-2} 5^{-2}, 2^{-3} 3^{-2})$  one recovers the BIK action given above.

- 
- [1] S. Bellucci, E. Ivanov and S. Krivonos, Phys. Rev. D **64**, 025014 (2001) [hep-th/0101195]. S. Bellucci, E. Ivanov and S. Krivonos, Phys. Lett. B **502**, 279 (2001) [hep-th/0012236].
- [2] J. Broedel, J. J. M. Carrasco, S. Ferrara, R. Kallosh and R. Roiban, “ $\mathcal{N} = 2$  Supersymmetry and U(1)-Duality,” Phys. Rev. D **85**, 125036 (2012) [arXiv:1202.0014 [hep-th]].
